# Supplementary material for: Solid-Electrolyte Interphase During Battery Cycling: Theory of Growth Regimes
Source: arXiv:2004.01458 ancillary file (2020-04-03)
Supplement: Supplementary file 1 [file Supporting_information.pdf]

# Supporting Information: Solid-Electrolyte Interphase During Battery Cycling: Theory of Growth Regimes

Lars von Kolzenberg,[1,2] Arnulf Latz,[1,2,3] and Birger Horstmann[1,2,3,*]

[1]*Institute of Engineering Thermodynamics,*
*German Aerospace Center (DLR) Pfaffenwaldring 38-40, 70569 Stuttgart (Germany)*

[2]*Helmholtz Institute Ulm (HIU), Helmholtzstraße 11, 89081 Ulm (Germany)*

[3]*Ulm University (UUlm), Albert-Einstein-Allee 47, 89081 Ulm (Germany)*

(Dated: April 3, 2020)

* birger.horstmann@dlr.de

## I. PARAMETRIZATION

State of charge $c_\mathrm{s}$ and open circuit voltage $U_0$ are related by the OCV-curve measured by Attia et al. [1] (see figure 3c in their work). We fit the curve with expression SI-1,

$$U_0 = \left(\frac{1.24 - c_\mathrm{s}/c_\mathrm{s,max}}{1.16}\right)^{2.92} \mathrm{V} \tag{SI-1}$$

with the maximum concentration $c_\mathrm{s,max} = Q_\mathrm{s,max}\rho_\mathrm{cb}/F$. Based on this relationship between charge and voltage, we calculate the baseline cycle for differential capacity analysis, $\frac{\mathrm{d}Q}{\mathrm{d}U_0}_\mathrm{baseline}$. For this, we rearrange equation SI-1 as $c_\mathrm{s}(U_0)$ and then take the derivative with respect to voltage. Additionally, we replace $c_\mathrm{s}$ with $Q_\mathrm{s}\rho_\mathrm{cb}/F$ and $c_\mathrm{s,max}$ with $Q_\mathrm{s,max}\rho_\mathrm{cb}/F$.

$$\frac{\mathrm{d}Q}{\mathrm{d}U_0}_\mathrm{baseline} = -313.5\,\mathrm{C/g/V}^{0.66} U_0^{-0.66} \tag{SI-2}$$

The OCV-curve can furthermore be subdivided into a linear part at high potentials (equation SI-3) and an exponential part at low potentials (equation SI-4).

$$Q_\mathrm{lin} = 129.62\mathrm{mA\,h\,g^{-1}} - 125.17\mathrm{mA\,h\,g^{-1}\,V^{-1}} \cdot V \tag{SI-3}$$

$$Q_\mathrm{exp} = 93.27\mathrm{mA\,h\,g^{-1}} \cdot \exp\left(-0.21\frac{FU_0}{RT}\right) \tag{SI-4}$$

We account for tunneling of electrons inside the SEI by introducing an apparent thickness $L'_\mathrm{app} = L_\mathrm{SEI} - L_\mathrm{tun}$. However, if the SEI is thinner than the typical tunneling range, $L_\mathrm{SEI} < L_\mathrm{tun}$, the apparent thickness becomes negative. We avoid this nonphysical behavior by introducing the continuous function SI-5,

$$L_\mathrm{app} = \frac{L'_\mathrm{app}}{2} + \sqrt[10]{\left(\frac{L'_\mathrm{app}}{2}\right)^{10} + L^2_\mathrm{app,0}}. \tag{SI-5}$$

Thereby, we employ a smooth transition between tunneling and diffusion limited growth with the limiting cases $L_\mathrm{app} \to 0$ for $L_\mathrm{SEI} < L_\mathrm{tun}$ and $L_\mathrm{app} = L_\mathrm{SEI} - L_\mathrm{tun}$ for $L_\mathrm{SEI} > L_\mathrm{tun}$.

We list the parameter of the model in table SI-1.

| Variable | Description | Value | Unit | Source |
|---|---|---|---|---|
| $U_1$ | Maximum Voltage during cycling | 1.2 | V | [1] |
| $U_2$ | Minimum Voltage during cycling | 0.01 | V | [1] |
| $Q_{\mathrm{s,nom}}$ | Nominal maximum capacity of carbon black | 200 | $\mathrm{mA\,h\,g^{-1}}$ | [1] |
| $Q_{\mathrm{SEI,0}}$ | Irreversible capacity loss of first cycle | 310 | $\mathrm{mA\,h\,g^{-1}}$ | [1] |
| $L_{\mathrm{SEI,0}}$ | SEI growth of first cycle | 2 | nm | [2] |
| $j$ | Intercalation current | 2-40 | $\mathrm{mA\,g^{-1}}$ | [1] |
| $A_{\mathrm{cb,m}}$ | Mass specific area of carbon black | 62 | $\mathrm{m^2\,g^{-1}}$ | [3] |
| $\rho_{\mathrm{cb}}$ | Density of carbon black | 1.4 | $\mathrm{g\,cm^{-3}}$ | [4] |
| $A_{\mathrm{cb}}$ | Volume specific area of carbon black | $86.8 \times 10^6$ | $\mathrm{m^2\,m^{-3}}$ | $A_{\mathrm{cb,m}} \cdot \rho_{\mathrm{cb}}$ |
| $Q_{\mathrm{s,max}}$ | Maximum capacity of carbon black | 218 | $\mathrm{mA\,h\,g^{-1}}$ | [1] |
| $c_{\mathrm{s,max}}$ | Maximum lithium concentration of carbon black | 3.16 | $\mathrm{mol\,L^{-1}}$ | $Q_{\mathrm{s,max}} \cdot \rho_{\mathrm{g}}/F$ |
| $V_{\mathrm{SEI}}$ | Mean molar volume of SEI species | $1.078 \times 10^{-5}$ | $\mathrm{m^3\,mol^{-1}}$ | $L_{\mathrm{SEI,0}} A_{\mathrm{cb,m}} F / Q_{\mathrm{SEI,0}}$ |
| $D_{\mathrm{Li}}$ | Diffusion coefficient of Li atoms inside the SEI | $1 \times 10^{-15}$ | $\mathrm{m^2\,s^{-1}}$ | Assumed |
| $c_{\mathrm{Li,0}}$ | Reference concentration of Li atoms at the anode-SEI interface | 1 | $\mathrm{mol\,L^{-1}}$ | Assumed |
| $\kappa_{\mathrm{Li^+,SEI}}$ | Lithium ion conductivity of the SEI | $1 \times 10^{-8}$ | $\mathrm{S\,m^{-1}}$ | Assumed |
| $j_{0,0}$ | Butler-Volmer rate constant for intercalation | $6.4 \times 10^{-7}$ | $\mathrm{A\,m^{-2}}$ | Fitted |
| $j_{\mathrm{SEI,0,0}}$ | Butler-Volmer rate constant for Li atom formation | $7.04 \times 10^{-5}$ | $\mathrm{A\,m^{-2}}$ | Fitted |
| $F$ | Faraday's constant | 96485 | $\mathrm{C\,mol^{-1}}$ | |
| $R$ | Universal gas constant | 8.314 | $\mathrm{J\,mol^{-1}\,K^{-1}}$ | |
| $T$ | Temperature | 303 | K | [1] |
| $\alpha_{\mathrm{SEI}}$ | Symmetry factor for Butler-Volmer | 0.22 | - | [5] |
| $\mu_{\mathrm{Li,0}}$ | Chemical reference potential of Lithium interstitial atoms inside the SEI | 17.4 | $\mathrm{kJ\,mol^{-1}}$ | Fitted |
| $L_{\mathrm{app,0}}$ | Reference apparent thickness for equation SI-5 | 0.05 | nm | Fitted |
| $L_{\mathrm{tunnel}}$ | Typical tunneling distance for electrons | 2.05 | nm | Fitted |

Table SI-1: List of model parameters for carbon black.

| Variable | Description | Value | Unit | Source |
|---|---|---|---|---|
| $A_{\mathrm{g,m}}$ | Mass specific area of graphite | 0.6 | $\mathrm{m^2\,g^{-1}}$ | [6] |
| $\rho_{\mathrm{g}}$ | Density of graphite | 2 | $\mathrm{g\,cm^{-3}}$ | [4] |
| $A_{\mathrm{g}}$ | Volume specific area of graphite | $1.2\times10^{6}$ | $\mathrm{m^2\,m^{-3}}$ | $A_{\mathrm{g,v}}\cdot\rho_{\mathrm{g}}$ |
| $Q_{\mathrm{s,max,g}}$ | Maximum capacity of graphite | 372 | $\mathrm{mA\,h\,g^{-1}}$ | [7] |
| $c_{\mathrm{s,max,g}}$ | Maximum lithium concentration of graphite | 7.71 | $\mathrm{mol\,l^{-1}}$ | $Q_{\mathrm{s,max,g}}\cdot\rho_{\mathrm{g}}/F$ |

Table SI-2: List of model parameters for graphite. Parameters not listed are equal to the carbon black parametrization shown in table SI-1

## II. TAFEL APPROXIMATION

For large overpotentials $\eta_{\mathrm{int}}$, we can approximate the Butler-Volmer equation 9 with the Tafel equation SI-6 ("+" for deintercalation, "-" for intercalation)

$$j_{\mathrm{int}} = \pm 2 j_0 e^{\pm\frac{F}{2RT}\eta_{\mathrm{int}}}. \tag{SI-6}$$

Using expression SI-6, we reformulate the exponential dependence of equation 23 on $\eta_{\mathrm{int}}$ as shown in equation SI-7,

$$e^{-\alpha_{\mathrm{SEI}}\frac{F}{RT}\eta_{\mathrm{int}}} = \left(\frac{j_{\mathrm{int}}}{2j_0}\right)^{2\alpha_{\mathrm{SEI}}} \propto j_{\mathrm{int}}^{2\alpha_{\mathrm{SEI}}}. \tag{SI-7}$$


[1] P. M. Attia, S. Das, S. J. Harris, M. Z. Bazant, W. C. Chueh, *J. Electrochem. Soc.* **2019**, *166*, E97–E106, doi:10.1149/2.0231904jes.

[2] W. Huang, P. M. Attia, H. Wang, S. E. Renfrew, N. Jin, S. Das, Z. Zhang, D. T. Boyle, Y. Li, M. Z. Bazant, B. D. McCloskey, W. C. Chueh, Y. Cui, *Nano Lett.* **2019**, *19*, 5140–5148, doi:10.1021/acs.nanolett.9b01515.

[3] S. Das, P. M. Attia, W. C. Chueh, M. Z. Bazant, *J. Electrochem. Soc.* **2019**, *166*, E107–E118, doi:10.1149/2.0241904jes.

[4] J. J. Kipling, J. N. Sherwood, P. V. Shooter, N. R. Thompson, *Carbon* **1964**, *1*, 321–328, doi:10.1016/0008-6223(64)90286-6.

[5] Y. Li, Y. Qi, *Energy Environ. Sci.* **2019**, 1286–1295, doi:10.1039/c8ee03586e.

[6] O. N. Shornikova, E. V. Kogan, N. E. Sorokina, V. V. Avdeev, *Russ. J. Phys. Chem. A* **2009**, *83*, 1022–1025, doi:10.1134/S0036024409060260.

[7] J. M. Tarascon, M. Armand, *Mater. Sustainable Energy Appl.* **2010**, *414*, 171–179, doi: 10.1142/9789814317665_0024.
